# Supplementary material for: FedMVP: Federated Multimodal Visual Prompt Tuning for Vision-Language Models
Source: arXiv:2504.20860 source file (2025-09-02)
Supplement: Supplementary file 1 [file parameters.tex]

\begin{table}[t]

    \centering
    \caption{{\textbf{\btoncap setting.}} Accuracies (\%) on client's local (seen) classes, base (seen) classes and new (unseen) classes. Harmonic mean (HM) is computed with Base and New class accuracies. Best number in each column is in bold.}
    \vspace{-.2cm}
    \scalebox{0.69}{
    \begin{tabular}{lcccc|ccc}
    \toprule
        
        \textbf{Methods} & \textbf{Prompts} & {Local} & {Base} & {New} & {HM} & {T. Params}\\ 
        \midrule
         
        ZS-CLIP \cite{clip} &hand-crafted &76.72	&70.51	&75.78	&\cellcolor[gray]{0.9}74.24 & 0 \\ 
        \midrule
        FedOTP \cite{fedotp} &\multirow{4}{*}{textual} &74.82 &65.22 &57.04 &\cellcolor[gray]{0.9}64.89 &16,384 \\
        FedKgCoOp \cite{kgcoop} & &78.38	&72.18	&75.87	&\cellcolor[gray]{0.9}75.39 &2048 \\
        PromptFL \cite{promptfl} & &\textbf{81.75}	&74.47	&71.70	&\cellcolor[gray]{0.9}75.74 &2048 \\
        FedTPG \cite{fedtpg} & &80.75	&73.68	&76.02	&\cellcolor[gray]{0.9}76.70  &4.2M\\
        \midrule
        FedCLIP \cite{fedclip}&visual &76.87 &71.04 &75.06 &\cellcolor[gray]{0.9}74.24 &0.52M  \\
        \midrule
        FedCoCoOp \cite{cocoop}&\multirow{3}{*}{textual+visual} &81.46	&73.76	&66.00	&\cellcolor[gray]{0.9}73.20 &35,360 \\
        
        FedMaPLe \cite{maple}& &81.63	&74.44	&70.62	&\cellcolor[gray]{0.9}75.29 &3.55M\\
         
        \method (Ours) & &80.80	&\textbf{74.50}	&\textbf{77.51}	&\cellcolor[gray]{0.9}\textbf{77.52} &19.3M \\

\bottomrule
    \end{tabular}}
    \label{tab:base2new}
    \vspace{-0.5cm}
\end{table}
